# Supplementary material for: Mitigating Hallucination in Visual Language Models with Visual Supervision
Source: arXiv:2311.16479 source file (2023-11-27)
Supplement: Supplementary file 1 [file X_suppl.tex]

\clearpage
\setcounter{page}{1}
\maketitlesupplementary

\section{Details on Data Construction}
\label{sec:detail_data}
In Section~\ref{sec:data}, we outline the process for constructing the RAI-30k dataset, which involves sending seed relationships and associated annotations to GPT-4. This section provides an in-depth explanation of the process.

Each time we construct a question-answer pair, we provide the following content in the input prompts: a directive indicating the nature of conversations to be generated (the system message), and the vision annotations exploited as the basis for forming such pairs. The detailed prompts are displayed in Table~\ref{tab:prompt_yes} and Table~\ref{tab:prompt_www}. We manually design different system prompts, and these prompts yield a multiplicity of question forms, including yes-or-no questions, and questions starting with what, how, where, etc.

To aid GPT-4 in comprehending the structure and context requisite for each specific type, we also supply a selection of examples in the prompt, and perform few-shot learning. This can also ensure that the yielded outputs could be automatically analyzed into question-answer combinations, which are rendered in the fixed format shown below. The system prompts and examples we use are organized in separate text files in supplementary as well.

\begin{spverbatim}
(Other analysis ...)
Question: <question>
Answer: <answer>
\end{spverbatim}

\begin{table*}[t]
  \centering
  \begin{tabularx}{\textwidth}{lX}
    \hline
    \multicolumn{2}{c}{\textbf{System Prompt}} \\ \hline
    \textbf{System}  & {You are an AI visual assistant, and you are seeing a single image. What you see are provided with IMAGE\_CONTENT, describing the same image you are looking at. IMAGE\_CONTENT contains general descriptions and the detailed objects in the image. If the position of a region or an object is provided. The positions are in the form of bounding boxes (x1, y1, x2, y2). The numbers are all floats ranging from 0 to 1, corresponding to the top left corner and bottom right corner in relative values.

Please generate a question-answer pair with a given topic. Only include questions that have definite answers, for example

(1) one can see the content in the image that the question asks about and can answer confidently;

(2) one can determine confidently from the image that it is not in the image.
Do not ask any question that cannot be answered confidently. Do not include bounding boxes in the conversation.

Your question and answer should concentrate on the relationship. You may ask about the item categories / item attributes / relationship between items.

Make make sure the question is logical. Please first give out your analysis and thinking, then generate one question-answer pair. The question should be a yes-or-no question.

If you think this relationship is not worth a question, please generate "skip" to skip this question.} \\ \hline
    \multicolumn{2}{c}{\textbf{Few Shot Examples}} \\ \hline
    \textbf{Human} & {IMAGE\_CONTENT

1. The image can be generally describe as:

   - a girl is looking at a blue clock

2. There are some objects in this image:

   - person [0.906, 0.984, 0.603, 0.976]
   
   - person [0.106, 0.121, 0.412, 0.800]
   
   - clock [0.406, 0.228, 0.612, 0.754]

3. There are some regional description that are overlapped with the subject and the object

   - a big blue clock [0.406, 0.228, 0.612, 0.751]
   
   - a girl in white dress [0.106, 0.121, 0.412, 0.902]
   
   - a girl in red jacket [0.906, 0.984, 0.603, 0.976]

Please generate the question-answer pair based on the following relation ship:

people (with bounding box [0.106, 0.121, 0.412, 0.800]) beside clock (with bounding box [0.406, 0.228, 0.612, 0.754])}\\
    \textbf{AI} & {According to the content, the girl besides the clock is wearing a white dress. So I will ask about this attribute.

Question: Is girl besides the clock wearing a white dress?

Answer: Yes, the girl besides the clock is wearing a white dress.} \\
    {} & {}\\ 
    \textbf{...} & {\#\#\# \{MORE EXAMPLES\}}\\ \hline
    \multicolumn{2}{c}{\textbf{Inputs}} \\ \hline
    \textbf{Human} & IMAGE\_CONTENT
    
1. The image can be generally describe as:

\#\#\# \{Fill in image captions\}

2. There are some objects in this image:

\#\#\# \{Fill in objects and bounding boxes\}

3. There are some regional description that are overlapped with the subject and the object

\#\#\# \{Fill in region descriptions\}

Please generate the question-answer pair based on the following relation ship:

\#\#\# \{Fill in a seed relation annotation\}\\
    \hline
  \end{tabularx}
  \caption{Prompt to generate yes-or-no question-answer pairs.}
  \label{tab:prompt_yes}
\end{table*}

\begin{table*}[t]
  \centering
  \begin{tabularx}{\textwidth}{lX}
    \hline
    \multicolumn{2}{c}{\textbf{System Prompt}} \\ \hline
    \textbf{System} & {You are an AI visual assistant, and you are seeing a single image. What you see are provided with IMAGE\_CONTENT, describing the same image you are looking at. IMAGE\_CONTENT contains general descriptions and the detailed objects in the image. If the position of a region or an object is provided. The positions are in the form of bounding boxes (x1, y1, x2, y2). The numbers are all floats ranging from 0 to 1, corresponding to the top left corner and bottom right corner in relative values.

Please generate a question-answer pair with a given topic. Only include questions that have definite answers, for example

(1) one can see the content in the image that the question asks about and can answer confidently;

(2) one can determine confidently from the image that it is not in the image.
Do not ask any question that cannot be answered confidently. Do not include bounding boxes in the conversation.

Your question and answer should concentrate on the given relationship. You may ask about the categories, attributes of the subject and object, or relationship between the subject and the object. Please ask what, how, where, which, why or who questions and answer it.

Make make sure the question is logical. Please first give out your analysis and thinking, then generate one question-answer pair. If you think this relationship is not worth a question, you can refuse to ask.} \\ \hline
    \multicolumn{2}{c}{\textbf{Few Shot Examples}} \\ \hline
    \textbf{Human} & {IMAGE\_CONTENT

1. The image can be generally describe as:

   - a girl is looking at a blue clock

2. There are some objects in this image:

   - person [0.906, 0.984, 0.603, 0.976]
   
   - person [0.106, 0.121, 0.412, 0.800]
   
   - clock [0.406, 0.228, 0.612, 0.754]

3. There are some regional description that are overlapped with the subject and the object

   - a big blue clock [0.406, 0.228, 0.612, 0.751]
   
   - a girl in white dress [0.106, 0.121, 0.412, 0.902]
   
   - a girl in red jacket [0.906, 0.984, 0.603, 0.976]

Please generate the question-answer pair based on the following relation ship:

people (with bounding box [0.106, 0.121, 0.412, 0.800]) beside clock (with bounding box [0.406, 0.228, 0.612, 0.754])}\\
    \textbf{AI} & {Question: Who is looking at the clock?

Answer: The girl in white dress is looking at the clock.} \\
    {} & {}\\ 
    \textbf{...} & {\#\#\# \{MORE EXAMPLES\}}\\ \hline
    \multicolumn{2}{c}{\textbf{Inputs}} \\ \hline
    \textbf{Human} & IMAGE\_CONTENT
    
1. The image can be generally describe as:

\#\#\# \{Fill in image captions\}

2. There are some objects in this image:

\#\#\# \{Fill in objects and bounding boxes\}

3. There are some regional description that are overlapped with the subject and the object

\#\#\# \{Fill in region descriptions\}

Please generate the question-answer pair based on the following relation ship:

\#\#\# \{Fill in a seed relation annotation\}\\
    \hline
  \end{tabularx}
  \caption{Prompt to generate wh-questions and their responses.}
  \label{tab:prompt_www}
\end{table*}

\begin{table*}[t]
  \centering
  \begin{tabularx}{\textwidth}{lX}
    \hline
    \multicolumn{2}{c}{\textbf{System Prompt}} \\ \hline
    \textbf{System}  & {The following question-answer pair is a conversation about an image. Please check what this conversation is about. It can be one of the following 3 categories:

1. The question contains a wrong obect category, and the answer corrects it.

2. The objects are right, but some attributes of one object is wrong (e.g., color, size, etc.)

3. The objects are right, but the relationship between them is wrong (e.g., relative position, action, etc.)

Please carefully analysis the question and answer, and choose the most suitable category.} \\ \hline
    \multicolumn{2}{c}{\textbf{Few Shot Examples}} \\ \hline
    \textbf{Human} & {Question: Is the bird standing on a tree?

Answer: No, the bird is standing next to a large body of water.}\\
    \textbf{AI} & {1. The question contains a wrong obect category, and the answer corrects it.}\\
    \\
    \textbf{Human} & {Question: Is the water in front of the person green?

Answer: No, the water in front of the person is very dark blue.}\\
    \textbf{AI} & {2. The objects are right, but some attributes of one object is wrong (e.g., color, size, etc.)}\\
    \\
    \textbf{Human} & {Question: Is the chair on the right side of the couch?
    
Answer: No, the chair is on the left side of the couch.}\\
    \textbf{AI} & {3. The objects are right, but the relationship between them is wrong (e.g., relative position, action, etc.)} \\ \hline
    \multicolumn{2}{c}{\textbf{Inputs}} \\ \hline
    \textbf{Human} & \#\#\# \{Our data here\}\\
    \hline
  \end{tabularx}
  \caption{Prompt to categorize question-answer pairs into different hallucination types.}
  \label{tab:prompt_subset}
\end{table*}

\section{Details on Benchmark Construction}
\label{sec:detail_bench}
We utilize similar prompts as in Section~\ref{sec:detail_data} to generate yes-or-no questions to construct RAH-30k. In order to further divide negative questions into the three hallucination types we proposed in Section~\ref{sec:benchmark}, we ask GPT-4 to conduct a text classification tasks and predict what each question-answer pair should belong to. Similarly, several examples are provided for GPT-4 to refer. The detailed prompt is shown in Table~\ref{tab:prompt_subset}.

% The categorization results from GPT-4 are not always correct, while we would like the benchmark to be precise itself before it can evaluate other models. To address this, we perform human-filter after the question-answer pairs are first categoried by GPT-4.
The classification outcomes provided by GPT-4 are sometimes imprecise. Nevertheless, for the efficient evaluation of other models, it is essential to establish a benchmark with high precision. To tackle this issue, we undertake a process of human filtering once the question-answer pairs have initially been classified by GPT-4.
More specifically,we employ a web-based tool to facilitate this process. When filtering for one hallucination type, all related questions are listed on the website, each accompanied by a relevant image and an interactive checkbox. If one question-answer pair is determined not to fall within this type, it can be quickly removed with a single click. We keep 500 samples after checking, and they are then archived to form a subset in our evaluation benchmark.

\section{Experiment Settings}
During training, we mainly follow the training configurations and hyper-parameters in LLaVA, regardless of what LVLM to train. When conducting visual instruction tuning with our conversation samples in RAI-30k, the multi-round conversation data is trained by masking the instructions and questions, and only supervise the answer tokens in each turn.
The learning rate is set as $2\times 10^{-5}$ with a cosine scheduler, and the batch size is 128. The models are trained for one epoch.
Our experiment are conducted on a single machine equipped with 8 A100 GPUs.

When training different LVLMs, we simply load their pretrained weights and then conduct instruction tuning with the same training settings. Moreover, these LVLMs involve different conversation templates as listed below. We strictly follow the original templates by replacing \verb|<image>|, \verb|<question>| and \verb|<answer>| with our conversations when formulating the input sequences.

\paragraph{LLaVA-LLaMA-2}
\begin{spverbatim}
[INST] <<SYS>> You are a helpful language and vision assistant. You are able to understand the visual content that the user provides, and assist the user with a variety of tasks using natural language. <</SYS>> <image> <question> [/INST] <answer> </s>
\end{spverbatim}

\paragraph{mPLUG-owl}
\begin{spverbatim}
The following is a conversation between a curious human and AI assistant. The assistant gives helpful, detailed, and polite answers to the user's questions.
Human: <image>
Human: <question>
AI: <answer>
\end{spverbatim}

\paragraph{InstructBLIP}
\begin{verbatim}
<image> <question> <answer>
\end{verbatim}
